# Supplementary material for: X-Field: A Physically Grounded Representation for 3D X-ray Reconstruction
Source: arXiv:2503.08596 source file (2025-03-11)
Supplement: Supplementary file 1 [file X_suppl.tex]

\clearpage
\setcounter{page}{1}
\maketitlesupplementary

\section*{Overview}
\begin{itemize}
    \item Detailed Derivations for Segment Lengths \S~\ref{sec:derivation}
    \item Implementation Details \S~\ref{sec:sup_implementation}:
    \begin{itemize}
        \item Dataset \S~\ref{sec:sup_dataset}
        \item Hyper parameters \S~\ref{sec:sup_hyperparam}
    \end{itemize}
    
    \item Additional Quantitative Results \S~\ref{sec:sup_quantitative}:

    \item Additional Qualitative Results \S~\ref{sec:sup_qualitative}:

    \item More Discussions \S~\ref{sec:sup_discussion}:
    \begin{itemize}
        \item Limitations \S~\ref{sec:sup_limitations}
        \item Ethics Considerations \S~\ref{sec:sup_ethicsconsiderations}
    \end{itemize}
\end{itemize}

\input{tables/all_compare_sup_view10}

\input{tables/all_compare_sup_view5}

\input{figs/tex/foot360}

\input{figs/tex/head360}

\input{figs/tex/jaw360}

\input{figs/tex/teapot360}

\section{Detailed Derivations for Segment Lengths}
\label{sec:derivation}
In this work, we define the ray space using normalized device coordinates (NDC) \cite{r2_gaussian}, providing a convenient framework for deriving explicit segment length formulas. In this space, the segment length \( l_i \) for each ellipsoid \(\mathbf{E}_i\) is calculated along the view direction \(\mathbf{d}\) of a given ray path.
Leveraging the orthographic property of NDC space, the 3D ellipsoid \(\mathbf{E}_i\) can be projected onto a 2D plane, forming an ellipse.
The segment lengths are then constrained within this 2D ellipse, with values outside the ellipse set to zero.

Our goal is to find the relationship between the segment length and the point $\mathbf{u} = (x, y, 0)$ on the ellipse traversed by the ray.
Below, we first derive the special value \( l_{\text{max}} \), which is the maximum distance a ray travels through the ellipsoid when originating from the center of the ellipse \cite{baer2005linear}.
Then, we use \( l_{\text{max}} \) as a bridge to express \( l_i \) for rays originating from other points on the ellipse.

Consider a ray originating from the center of the ellipse \( \mathbf{u_c} \) and traveling among direction \( \mathbf{d} \). The modeling of the ray is:
\(
\mathbf{R}(s) = \mathbf{u_c} + s\mathbf{d} \in \mathbb{R}^3,
\)
where \( s \) is a scalar parameter. Meanwhile, the ellipsoid centered at \( \mathbf{p_c} \) can be described as
\begin{equation}
(\mathbf{p} - \mathbf{p_c})^\top \mathbf{\Sigma}_{\text{3D}}^{-1} (\mathbf{p} - \mathbf{p_c}) = 1.
\end{equation}
Substituting \( \mathbf{p} = \mathbf{R}(s) \) into above equation, we have $s$ as in
\begin{equation}
(\mathbf{u_c} + s\mathbf{d} - \mathbf{p_c})^\top \mathbf{\Sigma}_{\text{3D}}^{-1} (\mathbf{u_c} + s\mathbf{d} - \mathbf{p_c}) = 1.
\end{equation}
In the NDC space, translating an object does not affect its geometric length. Therefore, without loss of generality, we can assume that $\mathbf{p_c}$ lies on $\mathbf{u_c}$, and then we have:
\begin{equation}
(\mathbf{u_c} + s\mathbf{d} - \mathbf{p_c})^\top \mathbf{\Sigma}_{\text{3D}}^{-1} (\mathbf{u_c} + s\mathbf{d} - \mathbf{p_c}) =
s^2 \mathbf{d}^\top \mathbf{\Sigma}_{\text{3D}}^{-1} \mathbf{d} =
1.
\end{equation}
Solving this simplified equation, we can obtain the roots:
\begin{equation}
s = \pm \frac{1}{\sqrt{A}}, \quad \text{where} \quad A = \mathbf{d}^\top \mathbf{\Sigma}_{\text{3D}}^{-1} \mathbf{d}.
\end{equation}
The segment length corresponding to $\mathbf{u_c}$ is the difference between the two roots: $l_{\text{max}} = |s_2 - s_1| = \frac{2}{\sqrt{A}}$.

Next, we consider a general point \( \mathbf{u} \) on the ellipse plane. The ray originating from \( \mathbf{u} \) in the direction \( \mathbf{d} \) can be represented by $\mathbf{R}(s) = \mathbf{u} + s\mathbf{d}$.
Similarly, we define \( \mathbf{a} = \mathbf{u} - \mathbf{p_c} \) and substitute \( \mathbf{R}(s) \) into the ellipsoid equation:
\begin{equation}
(\mathbf{a} + s\mathbf{d})^\top \mathbf{\Sigma}_{\text{3D}}^{-1} (\mathbf{a} + s\mathbf{d}) = 1.
\end{equation}
Expanding the equation results in:
\begin{equation}
s^2 \mathbf{d}^\top \mathbf{\Sigma}_{\text{3D}}^{-1} \mathbf{d} + 2s \mathbf{a}^\top \mathbf{\Sigma}_{\text{3D}}^{-1} \mathbf{d} + \mathbf{a}^\top \mathbf{\Sigma}_{\text{3D}}^{-1} \mathbf{a} = 1.
\end{equation}
For simplicity, we denote $B{=}\mathbf{a}^\top \mathbf{\Sigma}_{\text{3D}}^{-1} \mathbf{d}$ and $C{=}\mathbf{a}^\top \mathbf{\Sigma}_{\text{3D}}^{-1} \mathbf{a}$. Thus, the equation becomes $A s^2 + 2B s + C - 1 = 0$, whose roots are:
\begin{equation}
s_{1,2} = \frac{-B \pm \sqrt{B^2 - A (C - 1)}}{A}.
\end{equation}
The segment length can then be derived as:
\begin{equation}
l_i = |s_2 - s_1| = l_{\text{max}} \times \sqrt{1 - \left( \frac{C - B^2}{A} \right)}.
\end{equation}

\section{Implementation Details}
\label{sec:sup_implementation}
\subsection{Dataset}
\label{sec:sup_dataset}
% 这部分讲datasets，讲讲我们和其它方法是在什么样的数据集上做实验的，训练的视角和测试的视角是怎么选择的（5view和10view）。以及介绍我们out of distribution的视角是怎么来的。
We conduct experiments on the large-scale X3D~\cite{sax_nerf} dataset with multiple modalities across two categories: Human Organ (Chest, Head, Foot, Jaw, Pancreas, Abdomen, aneurism, Leg) and Synthetic Object (Bonsai, Teapot, Engine, Backpack, box, carp, Pelvis). The chest scans are sourced from LIDC-IDRI \cite{armato2011lung}, the pancreas scans from Pancreas-CT \cite{Roth2016}, and the remaining cases from SciVis \cite{scivisdata}. Following prior works \cite{x_gaussian, r2_gaussian, sax_nerf}, we employ the TIGRE tomography toolbox \cite{biguri2016tigre} to capture 512$\times$512 projections across a range of $0^\circ$ to $180^\circ$, including both in-distribution and out-of-distribution views. 

\noindent \textbf{View Distribution.}
For training, we uniformly capture 5, 10, 15, 25, and 50 views within $0^\circ$ to $180^\circ$. For testing, we randomly capture 50 views in the same range. 

\noindent \textbf{Out-of-Distribution Views.} We also evaluate the robustness of our method on out-of-distribution views. To construct these views, we apply a consistent algorithm across all cases. Specifically, for each case, we calculate the Oriented Bounding Box (OBB) \cite{gottschalk1996obb} of the trained ellipsoid distribution to determine its center and principal axis. Next, we select a direction \(\mathbf{d}\) orthogonal to this principal axis. Starting from the center, we move along \(\mathbf{d}\) by a radius \(r\) to establish the initial camera position. The camera then rotates $360^\circ$ around the principal axis to form the view distribution.
Due to differences in direction and radius, the resulting new view distribution is entirely distinct from both the training and testing sets. This setup comprehensively evaluates the model’s robustness and 3D consistency under unseen views.

% \subsection{Baseline Implementation Details}
% \label{sec:sup_base_implementation}
% % 这部分写sax nerf，xgaussian r2gaussian是在什么条件下跑出来的实验结果
% We implement the traditional FDK \cite{feldkamp1984practical} and SART \cite{andersen1984simultaneous} algorithms to reconstruct CT volumes from the dataset. Using TIGRE \cite{biguri2016tigre}, we render 2D X-ray projections from the reconstructed volumes at specified camera poses and compare them with ground truth to evaluate reconstruction fidelity. 

% For the R$^2$-Gaussian  \cite{r2_gaussian}, we utilize the official implementation with default settings. The method's novel rendering component is retained, but voxelization is omitted because it is designed for jointly optimizing reconstruct CT rather than based on result of novel view synthesis only. Similarly,  we evaluate TensoRF \cite{chen2022tensorf}, NAF \cite{zha2022naf}, SAX-NeRF \cite{sax_nerf}, and X-Gaussian \cite{x_gaussian} by running their official implementations with default hyperparameters. The NeRF-based methods are configured for 50,000 training epochs, while 3DGS-based methods, including R$^2$-Gaussian  and X-Gaussian, are trained for 10,000 epochs. All experiments are conducted on a single NVIDIA RTX A6000 GPU for fair and consistent comparisons.

\subsection{Hyper-parameters}
\label{sec:sup_hyperparam}
% 这部分讲我们调整了哪些参数 最后是哪一套参数跑出来的我们的结果
In our experiments, the position learning rate was set to an initial and final value of 0.0002, while the density and scaling learning rates were both initialized and maintained at 0.01 and 0.005, respectively. The structural dissimilarity loss weight ($\lambda_{\text{DSSIM}}$) was set to 0.25. To refine the density of kernels, a minimum density threshold of $1 \times 10^{-5}$ was applied. Densification was performed every 100 iterations, beginning at iteration 1000 and continuing until iteration 10,000. The total number of kernels was capped at 500,000 to balance computational efficiency with accuracy.

\section{Additional Quantitative Results}
\label{sec:sup_quantitative}

Tables \ref{tab:all_comparison_sup_10} and \ref{tab:all_comparison_sup_5} present the scene-wise quantitative results for 10-view and 5-view training data, respectively. In the 10-view setting (Table \ref{tab:all_comparison_sup_10}), our method achieves the best performance in most scenes across all metrics, including PSNR, SSIM, and LPIPS. Specifically, for challenging scenes such as the pancreas and bonsai, our method consistently outperforms all others, demonstrating its ability to handle complex structures effectively. The R$^2$-Gaussian  method performs well in certain scenes, such as the foot and engine, achieving competitive SSIM and LPIPS scores. However, our method maintains an edge in PSNR and overall quality, solidifying its superiority in reconstructing finer details.

In the 5-view scenario (Table \ref{tab:all_comparison_sup_5}), the performance gap between methods decreases due to the limited training data. Nonetheless, our method achieves the best results in most scenes, particularly excelling in the chest, bonsai, and teapot, where it surpasses other methods across all metrics. While the R$^2$-Gaussian  method demonstrates strong performance in specific scenes, our approach consistently proves to be more robust. These results underscore our method's adaptability to reduced training data while maintaining state-of-the-art performance.

\section{Additional Qualitative Results}
\label{sec:sup_qualitative}

\paragraph{Out-of-Distribution Results}
\label{sec:sup_novelview}
To further evaluate X-ray reconstruction capabilities, we rendered 360-degree images around the scene. We compared X-Gaussian, R$^2$-Gaussian , and our method with viewpoints being out-of-distribution in 5 different scenes, including foot (Figure \ref{fig:foot360}), head (Figure \ref{fig:head360}), jaw (Figure \ref{fig:jaw360}), and teapot (Figure \ref{fig:teapot360})
% and bonsai (Figure \ref{fig:bonsait360})
. 

Each figure presents five out-of-distribution views, with rows representing methods and columns corresponding to the same view. In the foot scene (Figure \ref{fig:foot360}), X-Gaussian exhibits black linear artifacts in views 3 and 4. While R$^2$-Gaussian  reconstructs the general foot structure, our method delivers smoother and more visually consistent results. In the head scene (Figure \ref{fig:head360}), X-Gaussian displays wave-like artifacts at the top of the head, whereas both R$^2$-Gaussian  and our method achieve improved overall reconstructions. Notably, our method captures finer details, showcasing superior reconstruction quality and generalization. Similarly, in the jaw (Figure \ref{fig:jaw360}), teapot (Figure \ref{fig:teapot360})
% , and bonsai (Figure \ref{fig:bonsait360}
) scenes, our method produces clearer and more complete reconstructions compared to the other approaches.

\section{More Discussions}
\label{sec:sup_discussion}

\subsection{Limitations}
\label{sec:sup_limitations}
Despite the fact that our X-Field marks a significant advancement in X-ray sparse view reconstruction, it is not without clearly declaring its limitations:

\begin{itemize}
    \item \textbf{The ellipsoid representation may not be the most efficient.} We use ellipsoids to capture the internal material distribution of objects; however, there could exist a more efficient form that can reduce the number of parameters while also requiring fewer elements to effectively learn the material distribution.
    
    \item \textbf{Lack of leveraging large model prior knowledge.} Many recent methods for sparse view reconstruction have utilized prior knowledge from large models to guide their learning processes. In our task, we didn't find a suitable large model for X-ray data to introduce into our framework. It is possible that some large-scale medical models could provide prior knowledge to enhance convergence speed and improve overall performance.
\end{itemize}

\subsection{Ethics Considerations}
\label{sec:sup_ethicsconsiderations}

Ethical considerations are critical in developing X-ray reconstruction technologies. Ensuring informed consent for transparent communication about and limitations of X-ray reconstruction methods is essential to respect privacy and prevent misrepresentation. Secure handling and storage of medical imaging data are paramount to safeguard against unauthorized access and misuse. Furthermore, recognizing the potential risks associated with the misuse of advanced imaging technologies, we emphasize the importance of establishing robust ethical guidelines to ensure their responsible application. Our commitment is to uphold the highest ethical standards in all aspects of X-ray reconstruction, protecting the integrity and confidentiality of patient data.
% \clearpage
{
    \small
    \bibliographystyle{ieeenat_fullname}
    \bibliography{main}
}
